# Supplementary material for: DPVI: A Dynamic-Weight Particle-Based Variational Inference Framework
Source: arXiv:2112.00945 source file (2021-12-02)
Supplement: Supplementary file 1 [file appendix.tex]

\section{More Experimental Results}

\section{Experiment Settings and Hyper-Parameter Tuning}
